# Supplementary material for: Mapping out the emergence of topological features in the highly alloyed topological Kondo insulators Sm$_{1-x}M_x$B$_6$ ($M$=Eu, Ce)
Source: arXiv:2108.11453 source file (2021-08-25)
Supplement: Supplementary file 1 [file SI_SmB6_PD_Aug23_2021.pdf]

# Supplemental Material for: Mapping out the emergence of topological features in the highly alloyed topological Kondo insulators $Sm_{1-x}M_xB_6$ ($M$=Eu, Ce)


Yishuai Xu,[1] Erica C. Kotta,[1] M. S. Song,[2] B. Y. Kang,[2] J. W. Lee,[2] B. K. Cho,[2] Shouzheng Liu,[1] Turgut Yilmaz,[3] Elio Vescovo,[3] Jonathan D. Denlinger,[4] Lin Miao,[5] and L. Andrew Wray[1,*]

[1]*Department of Physics, New York University, New York, New York 10003, USA*
[2]*School of Materials Science and Engineering, Gwangju Institute of Science and Technology (GIST), Gwangju 61005, Korea*
[3]*National Synchrotron Light Source II, Brookhaven National Lab, Upton, New York 11973, USA*
[4]*Advanced Light Source, Lawrence Berkeley National Laboratory, Berkeley, CA 94720, USA*
[5]*School of Physics, Southeast University, Nanjing, 211189, China*



(Dated: August 23, 2021)


## ADDITIONAL MODELING DETAILS

We implemented a tight binding model based on Ref. [1]. Orbital energies were modified to better match the $k_z{\sim}0$ experimental spectrum, with values of $\epsilon^f_{\Gamma_7} = \epsilon^f_{\Gamma_8} = 0.5$ eV and $\epsilon_d = 1.97$ eV. The crystal field energy hierarchy defined by $\epsilon^f_{\Gamma_7}$ and $\epsilon^f_{\Gamma_8}$ causes the topological band gap to be defined by the $\Gamma_8$ basis, in keeping with inspections of surface state spin helicity and core level resonance in recent literature [2–5]. The unhybridized $5d$ dispersion was set to match the sinusoidal-like overlay to ARPES data in Fig. 4(a,b) of Ref. [6], with the $X$ point band minimum 1.8 eV below the Fermi energy, and a 2.4 eV full dispersion along the Γ-X axis.

To account for strong correlations, we implemented a slave-Boson approach following Ref. [1], which reduces the dispersion of the f bands. In particular, we re-scaled the hopping matrix of $d-d$, $f-f$ and $d-f$ by a factor of 0.72, 0.08 and 0.28, respectively, where the $d-d$ rescaling is obtained from ARPES data. The $f-f$ and $d-f$ rescaling emerge from a single renormalization factor applied to the f-electron creation operator. The band gap of our model is 9 meV, roughly consistent with a lower bound estimate of the $T\sim$20K bulk band gap attributed in Ref. [7]. Shifting the $\Gamma_7$ spectator states downward (reducing $\epsilon^f_{\Gamma_7}$ by up to 10 meV) can increase the gap size with negligible consequences for the properties of interest in this investigation. Placing the chemical potential in the middle of the band gap gives an f-electron count that converges to $\angle n_f\rangle = 5.43$ at low temperature, which is close to the value observed in experiment [8]. Surface spectral functions are obtained from slab calculations, stacking the layers along the [001] (z-axis) direction with the number of layers $N_z = 80$.

With respect to the crystal field, we note that larger values of $\epsilon^f_{\Gamma_7}$ reduce the insulating gap size, and are difficult to accommodate without greatly (and nonphysically) increasing the $4f$ bandwidth. Smaller values of $\epsilon^f_{\Gamma_7}$ can preserve the same essential band features ($\Gamma_8$ topological gap, $\overline{H}$-point local band maxima, insulating gap compatible with Ref. [7]) provided that $\epsilon^f_{\Gamma_7} \gtrsim \epsilon^f_{\Gamma_8} - 0.015$ eV, roughly consistent with the recent attribution of $\epsilon^f_{\Gamma_7} = \epsilon^f_{\Gamma_8} - 0.02$ eV $\pm 0.01$ eV [10]. For $\epsilon^f_{\Gamma_7} < \epsilon^f_{\Gamma_8} - 0.015$ eV, it becomes challenging to simultaneously reproduce the $\overline{H}$-point local band maxima and ∼12 meV insulating gap, even when $4f$ bandwidth is treated as a free parameter. We emphasize that this discussion relates only to the role of the crystal field in this particular model, and should not be interpreted as a strong constraint on the crystal field energetics outside of this context.

### Surface modeling and the $\Gamma_7$ spectator band

Our surface models were augmented with the Kondo breakdown (KB) term proposed in Ref. [11], as well as a surface potential (Fig. 1). Both the KB and surface potential terms are applied to only the topmost layer in the slab simulation, and the surface potential term $U_{surf}$ is applied to both d- and f- orbitals. As shown in Fig. 1(a), without the Kondo breakdown (KB) and surface potential terms, the surface state Fermi momentum is $\sim 0.1\text{Å}^{-1}$, much smaller than the experimental value of $\sim 0.25\text{Å}^{-1}$. We also note that the f-band immediately beneath the Fermi level ($\Gamma_7$ symmetry) is a 'spectator band' that does not hybridize significantly with the low energy Dirac cone surface state. This can be clearly seen in the right panels of Fig.1(a-d), where the $\Gamma_7$ band has been removed by applying a 100 eV large potential term to the $\Gamma_7$ orbital. The simulations in Fig. 1 use a thin slab with $N_z = 10$ to make the $\Gamma_7$ bulk states sparse, so that the surface state can be seen dispersing through them.

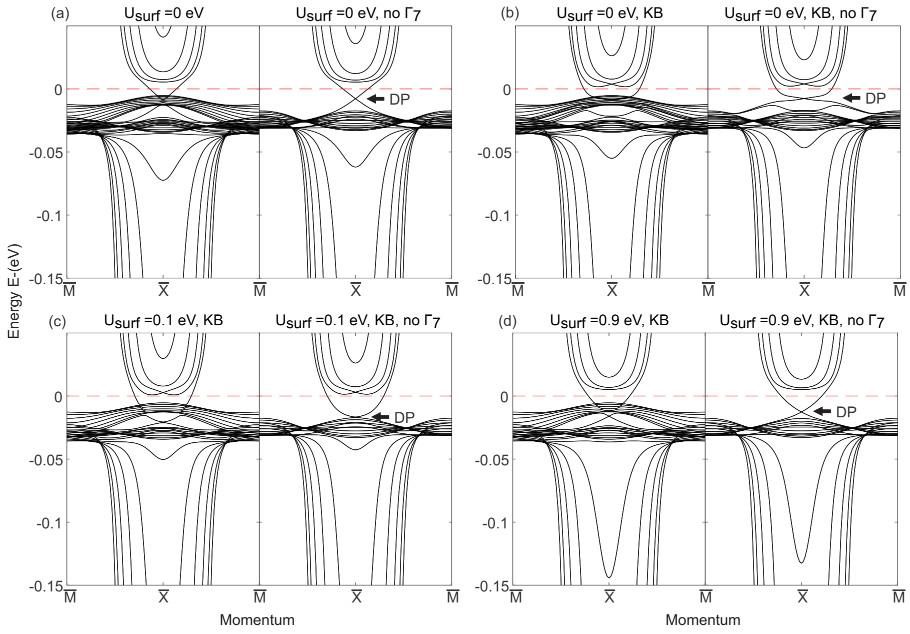


FIG. 1. Kondo breakdown and surface potential. Slab calculations are shown (left) with and (right) without the $\Gamma_7$ orbital for scenarios with (a) an unmodified surface, (b) Kondo breakdown at the surface but no Coulomb perturbation (U=0), (c) Kondo breakdown and a U=0.1 eV surface potential, and (d) Kondo breakdown and a U=0.9 eV surface potential.

Symmetries of the bulk conduction and valence bands are summarized in Fig. 2. The $\Gamma_7$ valence band is found to have negligible hybridization with the $5d$ band [see Fig. 2(b)], consistent with the attribution that it is not significantly involved in the opening of the $4f/5d$ topological hybridization gap. The valence band curve amplitude does not exceed 0.22%. The bulk Berry's phase $\phi_B$ of each band is plotted in Fig. 2(c), following the definition introduced in Ref. [9]. This metric was defined to assesses bulk symmetry inversion with respect to Majorana Fermion emergence in proximity-induced superconductivity, with the $\phi_B < \pi$ region designated as topologically nontrivial. Though both bands demonstrate phase evolution, the phase of the conduction band deviates from the valence band in a pattern that resembles the onset of hybridization with the $5d$ band, with a common inflection point at $\sim 0.5 \times \pi/a$ indicated by black arrows in Fig. 2(b-c). For representational convenience, the Berry's phase integral is conducted along a circular path through momentum space, rather than along a constant energy path.

The surface state dispersion changes when a KB and surface potential term are included as shown in Fig. 1(b-d). The KB term leaves the Dirac point buried in the $\Gamma_7$ band, but greatly increases the Fermi momentum and Fermi velocity of the upper Dirac cone, bringing them in reasonable correspondence with the experiment. The low Dirac velocity and shallow binding energy of the Dirac point are attractive features of the KB picture, with respect to STM [7], but are invisible to the simulated ARPES spectral function (Fig 4). Note that the surface state dispersion in Fig. 1(b, left) curls away from the $\Gamma_7$ band, giving the misimpression that there is strong hybridization with the bulk $\Gamma_7$ band, however this is not the case, as the same features are observed when the $\Gamma_7$ band is removed in Fig. 1(b, right). The surface state at the Fermi level in Fig. 1(b) has the same spin chirality with or without $\Gamma_7$, and each wavefunction projects 89% onto the alternate scenario.

A similar surface spectrum can be obtained by applying a positive surface potential of 0.05 eV $<$ U$_{surf}$ $<$ 1 eV. This occurs as a result of f-orbital states in the top quintuple layer being shifted above the Fermi level, and exerting a hybridization-derived level repulsion effect on the surface state. We have used U$_{surf}$=0.5 eV in the main text for convenience, so that the Dirac point is visible outside of the $\Gamma_7$ continuum, but the ARPES spectral function does not readily discern between the U$_{surf}$=0 and 0.05 eV $<$ U$_{surf}$ $<$ 1eV regimes (see Fig. 4).

Our adoption of the U$_{surf} > 0$ regime is physically motivated by two factors:

(1) There is a very strong correlation between B-termination and surface state spectral intensity in surface surveys that we have performed using ARPES spectromicroscopy, suggesting that B-terminated regions will be more strongly represented in the spectral function. The B-termination induces a positive surface potential, and is associated with surface state dispersions and Fermi contours that resemble both our model and earlier ARPES measurements [12]. Modeling in Ref. [12] effectively adopts the same $U > 0$ paradigm as our investigation, with the positive surface

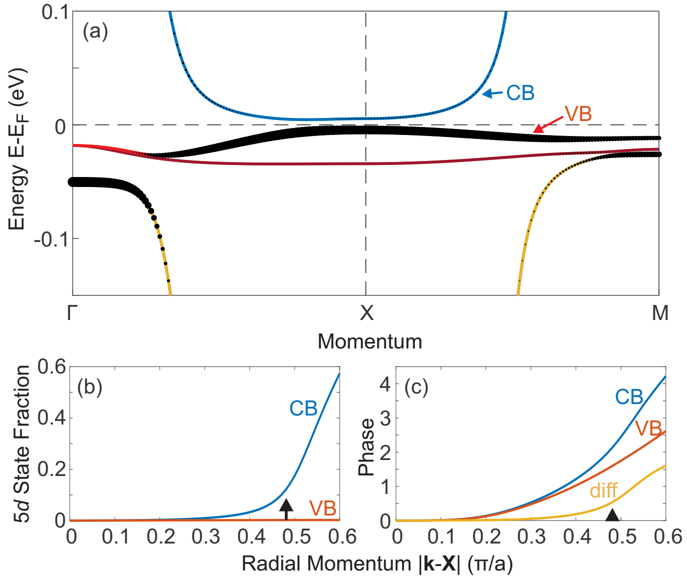


FIG. 2. Conduction and valence symmetries and topology. (a) The conduction band (CB) and valence band (VB) are identified on tight binding model band structure near the X-point symmetry inversion, with the $\Gamma_7$ orbital component indicated by the radius of overlaid black circles. (b) The $5d$ state component is shown for the conduction and valence bands as a function of momentum displacement from the X-point in the $k_z$=0 plane. (c) The bulk Berry's phase $\phi_B$ defined in Ref. [9] is shown as a function of momentum displacement from the X-point. Black arrows indicate an inflection point in $5d$ orbital weight of the conduction band, and in the Berry's phase difference between the conduction band and valence band.

potential resulting in localized states above the Fermi level, while the topological surface state primarily occupies the second Sm layer of the crystal [12].

(2) We wish to avoid confusion about the role of the $\Gamma_7$ band with respect to the topological state. In our model, the U=0 band structure has the superficial appearance of strong hybridization between the surface state and the $\Gamma_7$ band, as the surface state appears to curl away from the bulk valence band states in Fig. 5(b,left). This is highly misleading, as in actuality, the 'curling' dispersion anomaly is a coincidental feature that is unrelated to the $\Gamma_7$ band. The surface dispersion is essentially unchanged when the $\Gamma_7$ valence band is removed from the model Hamiltonian in Fig. 5(b,right).

## Spectral function and temperature

To simulate the interplay of temperature with f-electron coherence, we added a temperature dependent imaginary self energy term to the tight binding Hamiltonian for spectral function simulations. The self energy term applied to the d orbitals was constant, and a temperature dependent term based on Ref. Ref. [13] is applied to the f orbital bases. With the self energy term, the Green's function is

$$G(\omega, k) = \frac{1}{\omega - \mathcal{H}(k)} = \frac{1}{\omega - \mathcal{H}_k + i\Gamma_d + i\Gamma_f(T)} \tag{1}$$

where $\mathcal{H}_k$ is the tight binding Hamiltonian, and $\Gamma_d$ and $\Gamma_f$ are matrices containing the self energy terms for the 5d- and 4f-orbitals, respectively. The constant self energy for the $5d$ band is set to 5meV, and for the 4f band we used the raw $4f$-band energy widths fitted approximately at the momentum space X-point in Fig. 2(a) of Ref. [13]. For the temperatures $T$=6, 40, 80, 120 and 180K considered in our experiments, the $4f$-band self energy values are 14, 20, 28, 37 and 49 meV respectively. The width is not strictly required to go to zero at low temperature, as the fitted features are at non-zero binding energy, and all $SmB_6$ crystals feature some disorder. However, non-intrinsic factors of note include the imperfect z-axis momentum resolution, possible contributions from multiple near-degenerate bands, and the Gaussian-like experimental resolution. In this context, it is useful to note that sub-dominant broadening factors have reduced significance in a Voigt function, and the $\delta E \sim$7 meV energy resolution in Ref. [13] is expected to contribute just 1.4 meV to the f-electron feature width at half maximum (fwhm) at the crossover temperature of T=120K (considering a Voigt function with 37 meV fwhm).

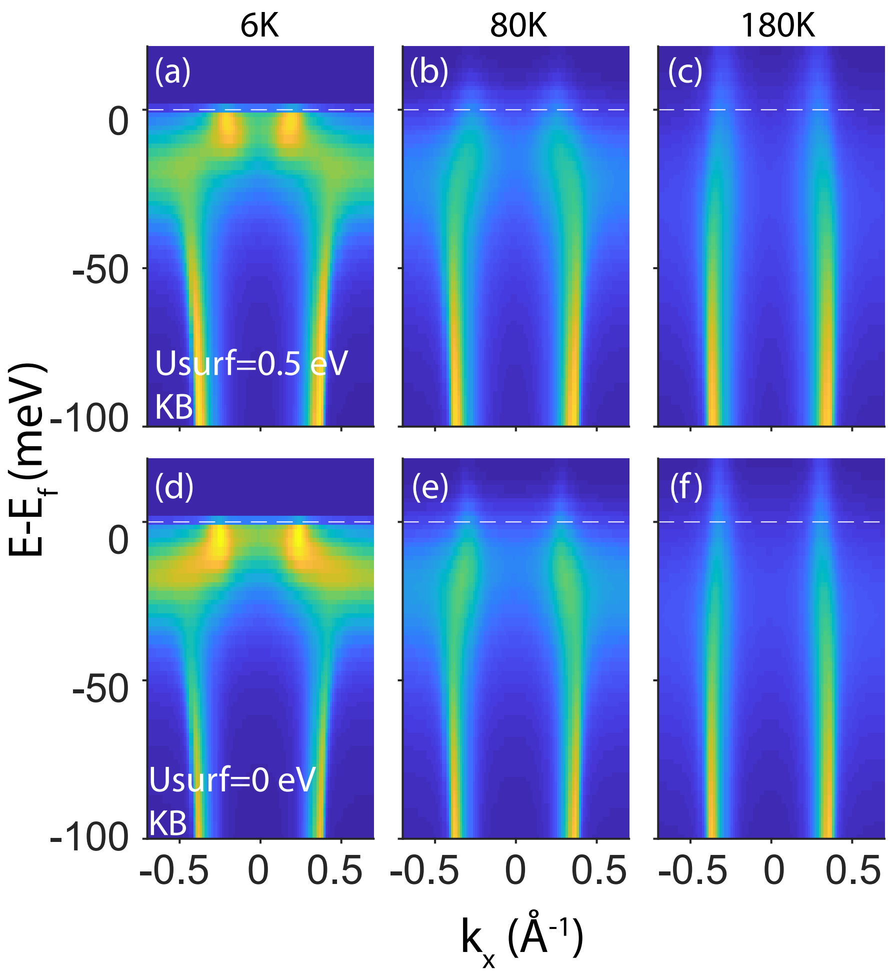


FIG. 3. Similar spectral functions with different surface potentials. (a-c) Spectral function with a surface potential $U_{surf}$=0.5 eV and a Kondo breakdown term at $T$ =6, 80 and 180K. (d-f) Corresponding spectral function with only Kondo breakdown, but no surface potential term.

To obtain the spectral function, we use the following relation,

$$A(\omega, k) = -\frac{1}{\pi}\sum_i \mathrm{Im}(\langle\psi_i| G(\omega, k) |\psi_i\rangle) \tag{2}$$

where photoemission matrix elements are encoded in the $|\psi_i\rangle$ vectors. As modeling of orbital photoemission matrix elements is not entirely reliable, we have performed a 'symmetry blind' sum over $|\psi_i\rangle$ states that separately index the single-site orbital basis, with relative amplitudes of 0.98 and 0.02 $5d$- and $4f$-orbitals respectively. The intersite structure of these $|\psi\rangle$ states is step function-like, with a constant amplitude and z-independent phase within 3 unit cells of the surface, and an amplitude of 0 in deeper layers of the crystal.

The significance of the two-gap picture with respect to thermalization is explored in Fig. 5, through comparison with an alternate model in which the $\Gamma_7$ band has been shifted to larger binding energy. In this alternate picture, insulating and topological gaps are accounted for via the $\Gamma_8$ band. The f-electron creation operator has been reduced by a further $\sqrt{2}$ factor to set the insulating gap to the a large but still reasonable value of 12 meV, which is the approximate zero-temperature value from Ref. [7]. As expected for this gap size, the surface state is already difficult to observe at an imaginary self energy of $Im(\Sigma) = 10$ meV [Fig. Fig. 5(h)], and vanishes well before the $Im(\Sigma) \sim 40$ meV threshold associated with surface state loss in Ref. [13, 14]. Moreover, the velocity lost to the $4d$ band is proportional to the $4f$ renormalization factor, and is too small by a factor of $\sqrt{2}$ in this picture.

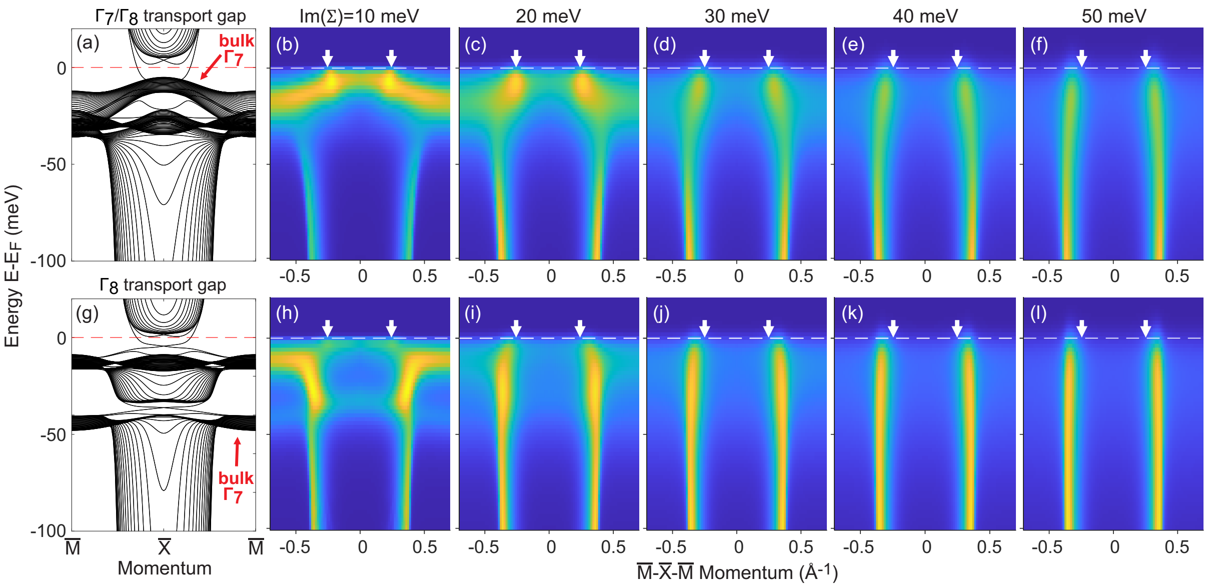


FIG. 4. Spectral function comparison with a $\Gamma_8$-only model. (a) The 2D slab band structure with Kondo breakdown and no surface potential (U=0). (b-f) Spectral evolution of the panel (a) model as a function of $4f$ self energy, with the surface state Fermi momentum indicated by white arrows. (g-l) the band structure and spectral function are shown for a $\Gamma_8$-only model, in which the $\Gamma_7$ band has been shifted to lower energy, and $4f$ hopping has been reduced by a factor of 2.

## SURFACE-NORMAL MOMENTUM RESOLUTION

It is worth noting that the fitted $k_z$ resolution of $\delta k_z$=0.57$\mathring{A}^{-1}$ is unusually poor, and inverts to a very small value $\sim$2$\mathring{A}$ (=1/$\delta k_z$) if interpreted as the skin depth of the measurement. Factoring in the $\sim$22° photoemission angle, the expected surface-normal inelastic mean free path of an electron excited at h$\nu$=21 eV is roughly 4$\mathring{A}$ (similar to one $SmB_6$ unit cell), and varies widely by material [15]. A shorter value in the present context may be understood by noting that topologically inverted bulk bands of the sort investigated here are believed to feature relatively poor $k_z$ resolution, due to large gradients in the bulk wavefunction where it overlaps with surface states in the outermost monolayers of a crystal [16]. Additionally, $4f$ compounds are known for particularly strong elastic (or quasielastic) scattering of photoelectrons derived from near the Fermi level [17], which will also negatively impact the effective penetration depth.

## ADDITIONAL SAMPLE CHARACTERIZATION

X-ray diffraction (XRD) curves for the highly alloyed Ce 50 and Eu 30 samples are shown in Fig. 5, and show an $SmB_6$ structure with no evidence of impurity phases. Additional XRD characterization of lower-doped samples can be found in the Supplemental Material to Ref. [14], along with extensive sample characterization data of other kinds. The trend of the fitted lattice parameters follows Vegard's law. For $Sm_{1-x}Eu_xB_6$, the fitted values are a = 4.1398, 4.1424 and 4.1437 $\mathring{A}$ for x=0.2, 0.3, and 0.4 respectively. ARPES data on the x=0.4 sample are excluded from this study, as the spectral quality was insufficient for high quality fitting. Low temperature coherence phenomena are not observed within the spectra, but this has little meaning with respect to the phase diagram. For $Sm_{1-y}Ce_yB_6$, the values are a = 4.1302, 4.1361, and 4.1399 $\mathring{A}$ for x=0.1, 0.3, and 0.5, respectively.

---

* lawray@nyu.edu; Corresponding author

[1] Pier Paolo Baruselli and Matthias Vojta, "Scanning tunneling spectroscopy and surface quasiparticle interference in models for the strongly correlated topological insulators $SmB_6$ and $PuB_6$," Phys. Rev. B **90**, 201106(R) (2014).
[2] M. Sundermann, H. Yavaş, K. Chen, D. J. Kim, Z. Fisk, D. Kasinathan, M. W. Haverkort, P. Thalmeier, A. Severing, and L. H. Tjeng, "4f crystal field ground state of the strongly correlated topological insulator $SmB_6$," Phys. Rev. Lett. **120**,

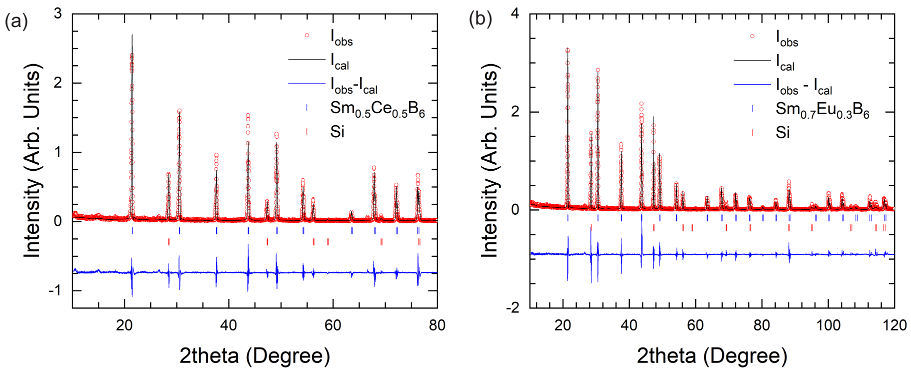


FIG. 5. Powder X-ray diffraction spectra of highly alloyed (a) Ce 50 and (b) Eu 30 samples show no impurity phase. All meaningful features are associated with the $SmB_6$ structure.

016402 (2018).

[3] Pier Paolo Baruselli and Matthias Vojta, "Distinct topological crystalline phases in models for the strongly correlated topological insulator $SmB_6$," Phys. Rev. Lett. **115**, 156404 (2015).

[4] Markus Legner, Andreas Rüegg, and Manfred Sigrist, "Surface-state spin textures and mirror chern numbers in topological kondo insulators," Phys. Rev. Lett. **115**, 156405 (2015).

[5] Pier Paolo Baruselli and Matthias Vojta, "Spin textures on general surfaces of the correlated topological insulator $SmB_6$," Phys. Rev. B **93**, 195117 (2016).

[6] Jonathan D. Denlinger, James W. Allen, Jeong-Soo Kang, Kai Sun, Byung-II Min, Dae-Jeong Kim, and Zachary Fisk, "$SmB_6$ photoemission: Past and present," in *Proceedings of the International Conference on Strongly Correlated Electron Systems (SCES2013)* (2014) https://journals.jps.jp/doi/pdf/10.7566/JPSCP.3.017038.

[7] Harris Pirie, Yu Liu, Anjan Soumyanarayanan, Pengcheng Chen, Yang He, M. M. Yee, P. F. S. Rosa, J. D. Thompson, Dae-Jeong Kim, Z. Fisk, Xiangfeng Wang, Johnpierre Paglione, Dirk K. Morr, M. H. Hamidian, and Jennifer E. Hoffman, "Imaging emergent heavy dirac fermions of a topological kondo insulator," Nat. Phys. **16**, 52–56 (2020).

[8] Masaichiro Mizumaki, Satoshi Tsutsui, and Fumitoshi Iga, "Temperature dependence of sm valence in $SmB_6$ studied by x-ray absorption spectroscopy," Journal of Physics: Conference Series **176**, 012034 (2009).

[9] Pavan Hosur, Pouyan Ghaemi, Roger S. K. Mong, and Ashvin Vishwanath, "Majorana modes at the ends of superconductor vortices in doped topological insulators," Phys. Rev. Lett. **107**, 097001 (2011).

[10] "Resonant inelastic x-ray scattering investigation of the crystal-field splitting of $Sm^{3+}$ in $SmB_6$," **100**, 241107(R) (2019).

[11] Victor Alexandrov, Piers Coleman, and Onur Erten, "Kondo breakdown in topological kondo insulators," Phys. Rev. Lett. **114**, 177202 (2015).

[12] Patrik Thunström and Karsten Held, "Topology of $SmB_6$ determined by dynamical mean field theory," Phys. Rev. B **104**, 075131 (2021).

[13] J. D. Denlinger, J. W. Allen, J. S. Kang, K. Sun, J. W. Kim, J. H. Shim, B. I. Min, Dae-Jeong Kim, and Z. Fisk, "Temperature dependence of linked gap and surface state evolution in the mixed valent topological insulator $SmB_6$," (2014), arXiv:1312.6637 [cond-mat.str-el].

[14] Lin Miao, Chul-Hee Min, Yishuai Xu, Zengle Huang, Erica C. Kotta, Rourav Basak, M. S. Song, B. Y. Kang, B. K. Cho, K. Kißner, Friedrich Reinert, Turgut Yilmaz, Elio Vescovo, Yi-De Chuang, Weida Wu, Jonathan D. Denlinger, and L. Andrew Wray, "Robust surface states and coherence phenomena in magnetically alloyed $SmB_6$," Phys. Rev. Lett. **126**, 136401 (2021).

[15] M. P. Seah and W. A. Dench, "Quantitative electron spectroscopy of surfaces: A standard data base for electron inelastic mean free paths in solids," Surface and Interface Analysis **1**, 2–11 (1979).

[16] L. Andrew Wray, Suyang Xu, Yuqi Xia, Dong Qian, Alexei V. Fedorov, Hsin Lin, Arun Bansil, Liang Fu, Yew San Hor, Robert J. Cava, and M. Zahid Hasan, "Spin-orbital ground states of superconducting doped topological insulators: A majorana platform," Phys. Rev. B **83**, 224516 (2011).

[17] Shin-ichi Fujimori, Takuo Ohkochi, Ikuto Kawasaki, Akira Yasui, Yukiharu Takeda, Tetsuo Okane, Yuji Saitoh, Atsushi Fujimori, Hiroshi Yamagami, Yoshinori Haga, Etsuji Yamamoto, and Yoshichika Ōnuki, "Electronic structures of ferromagnetic superconductors $uge_2$ and ucoge studied by angle-resolved photoelectron spectroscopy," Phys. Rev. B **91**, 174503 (2015).
